# Supplementary material for: Calibration and simulation of ionization signal and electronics noise in the ICARUS liquid argon time projection chamber
Source: arXiv:2407.11925 source file (2024-08-05)
Supplement: Supplementary file 1 [file equalization_appendix.tex]

\begin{figure}[]
    \centering
    \includegraphics[width=\textwidth]{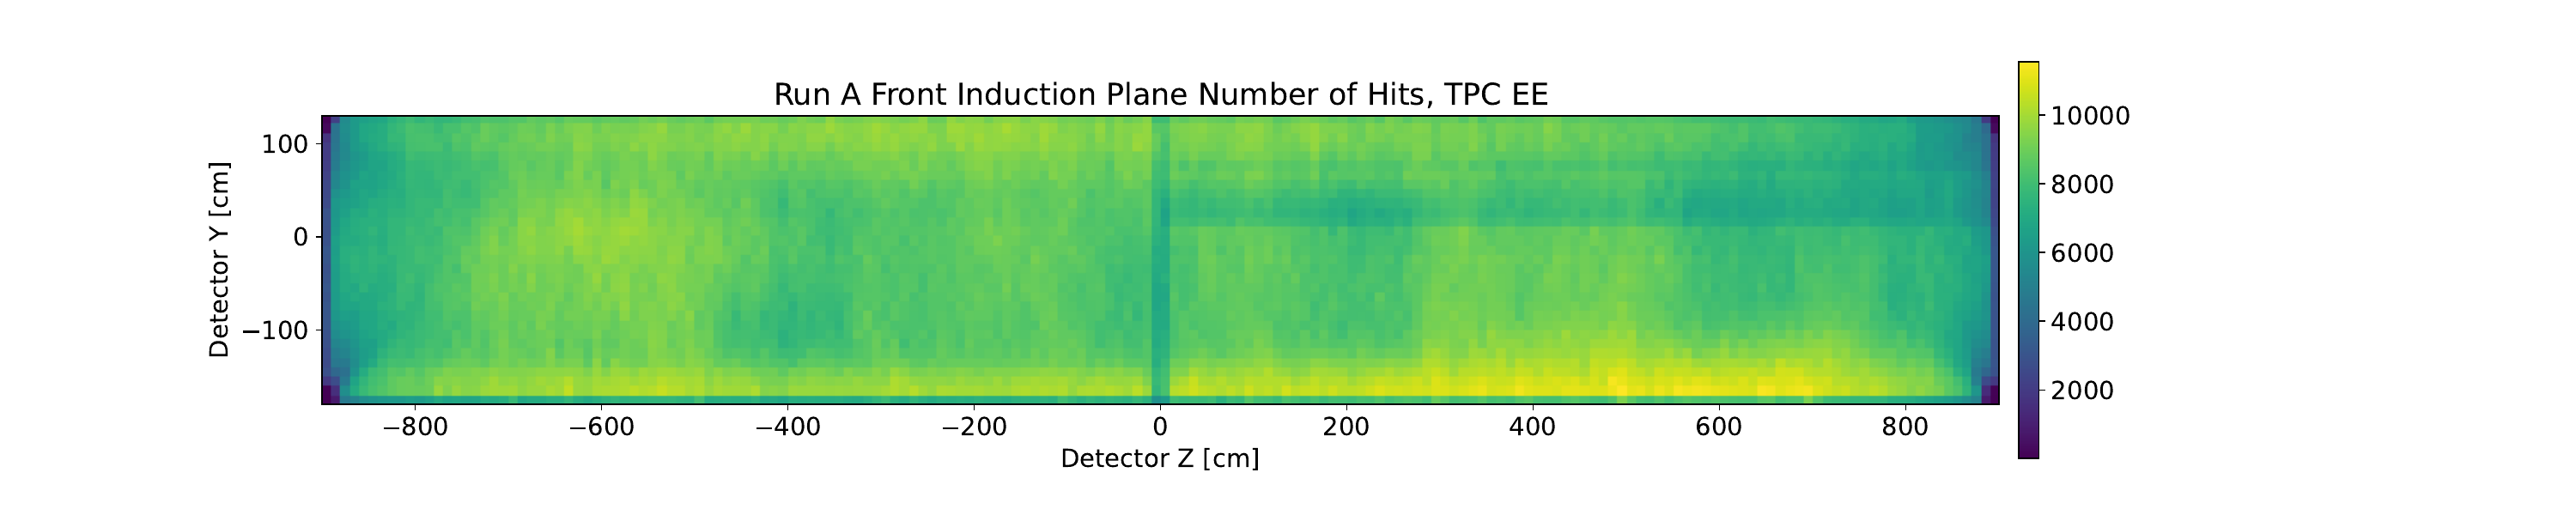}
    \includegraphics[width=\textwidth]{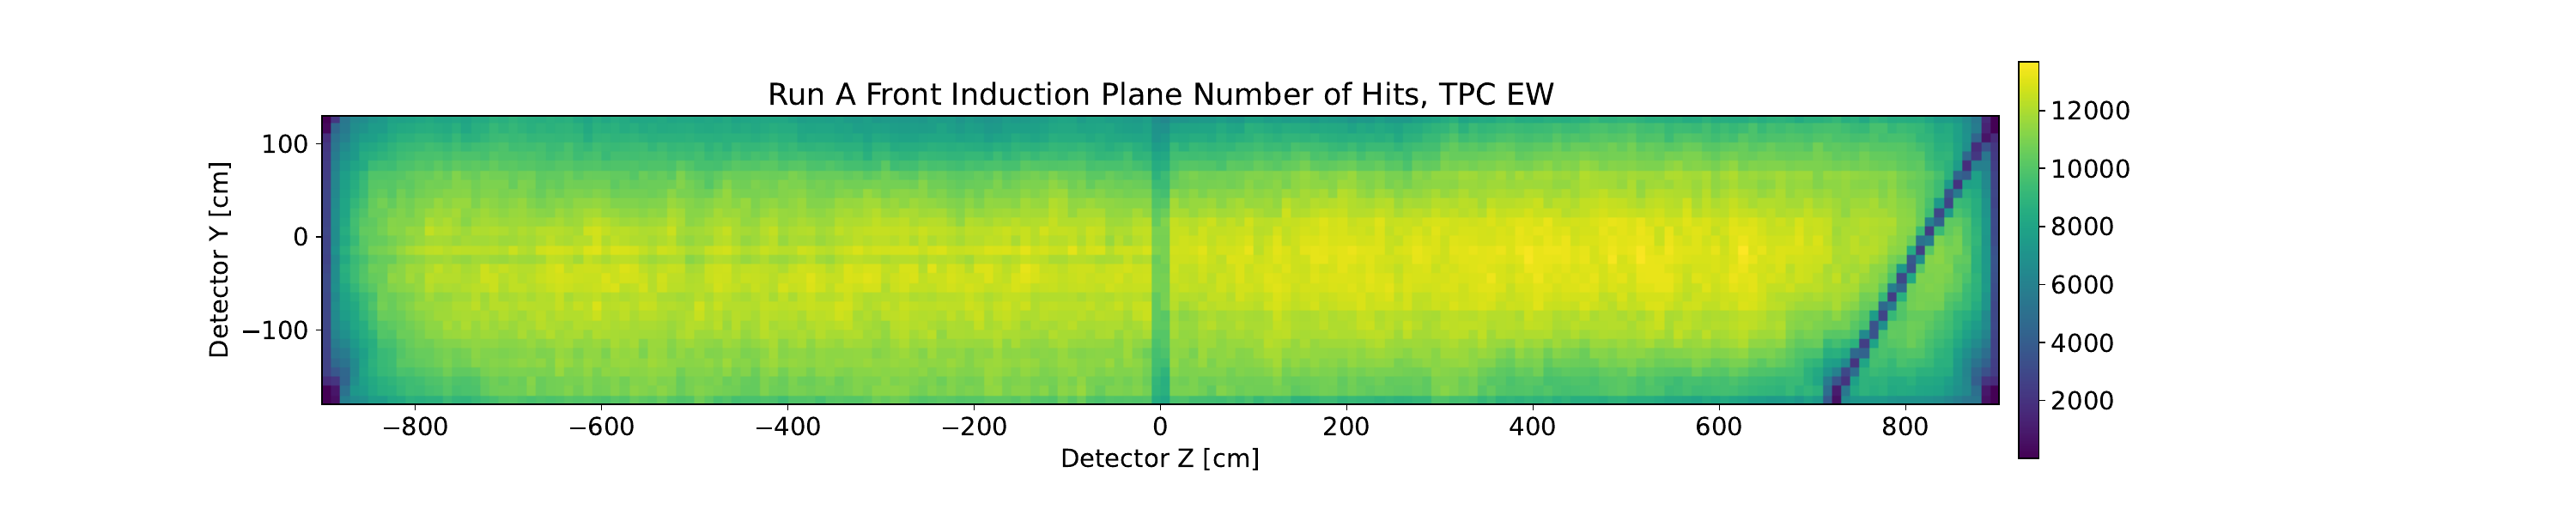}
    \includegraphics[width=\textwidth]{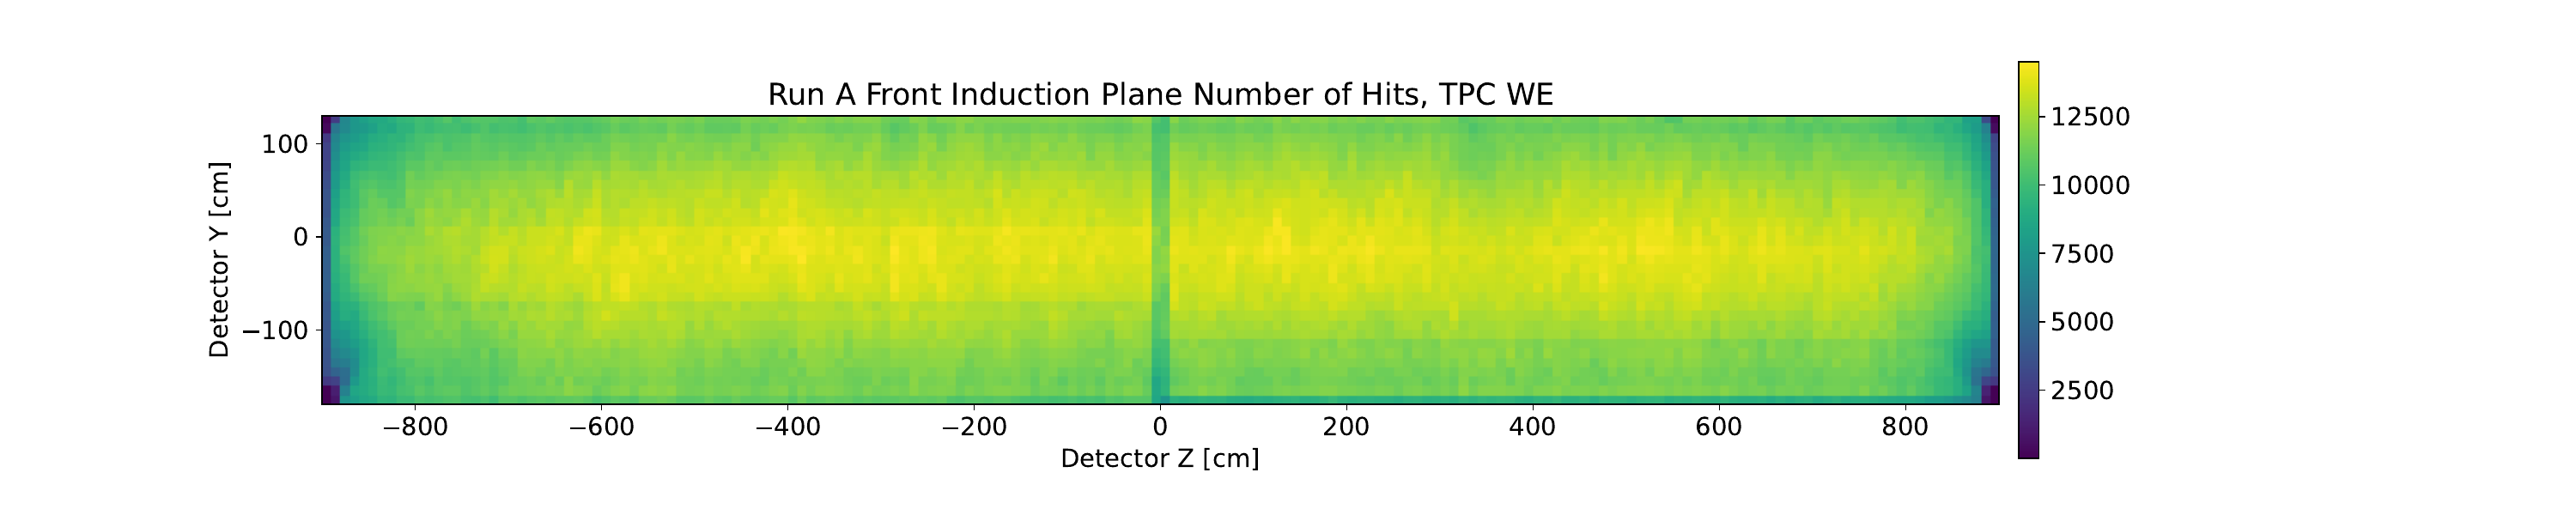}
    \includegraphics[width=\textwidth]{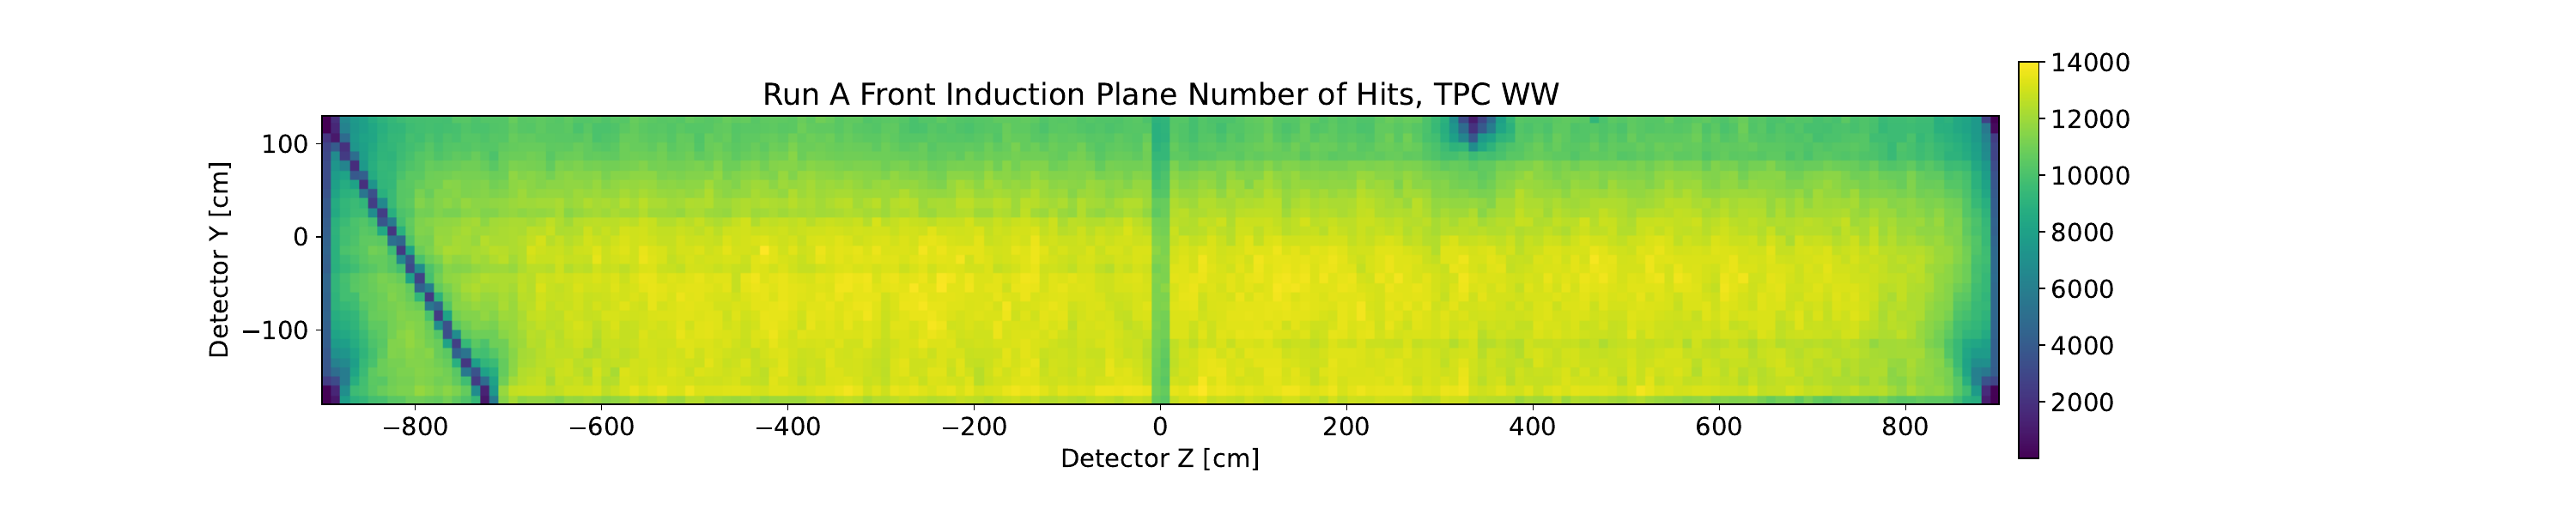}
    \caption{Number of depositions in $10\times$\SI{10}{\centi\meter} bins in each of the ICARUS TPCs on the front induction plane across the Run A dataset.}
    \label{fig:w=runAInd0N}
\end{figure}

\begin{figure}[]
    \centering
    \includegraphics[width=\textwidth]{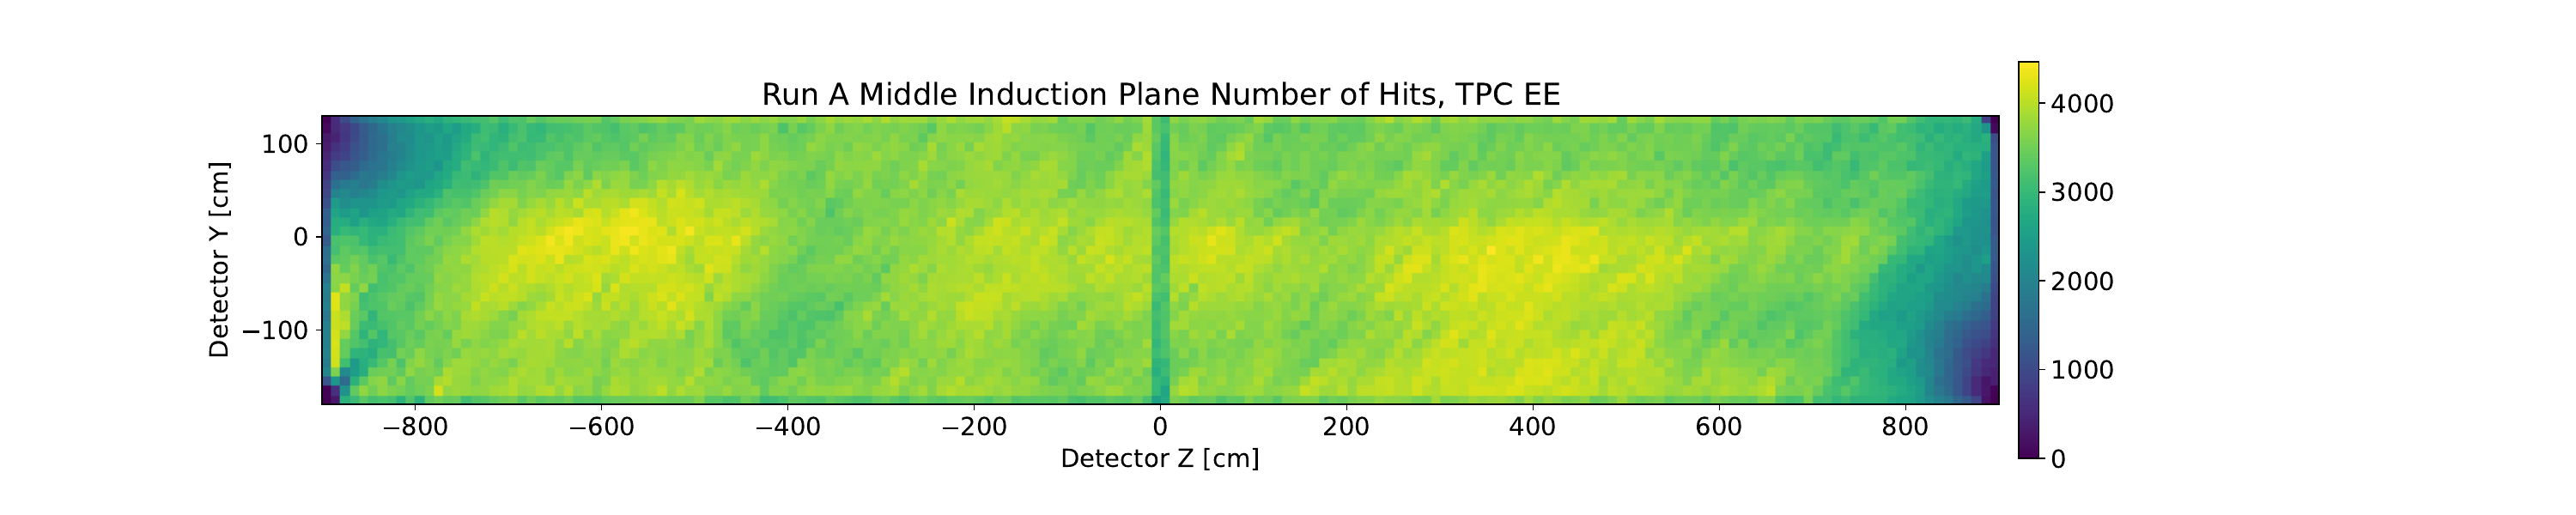}
    \includegraphics[width=\textwidth]{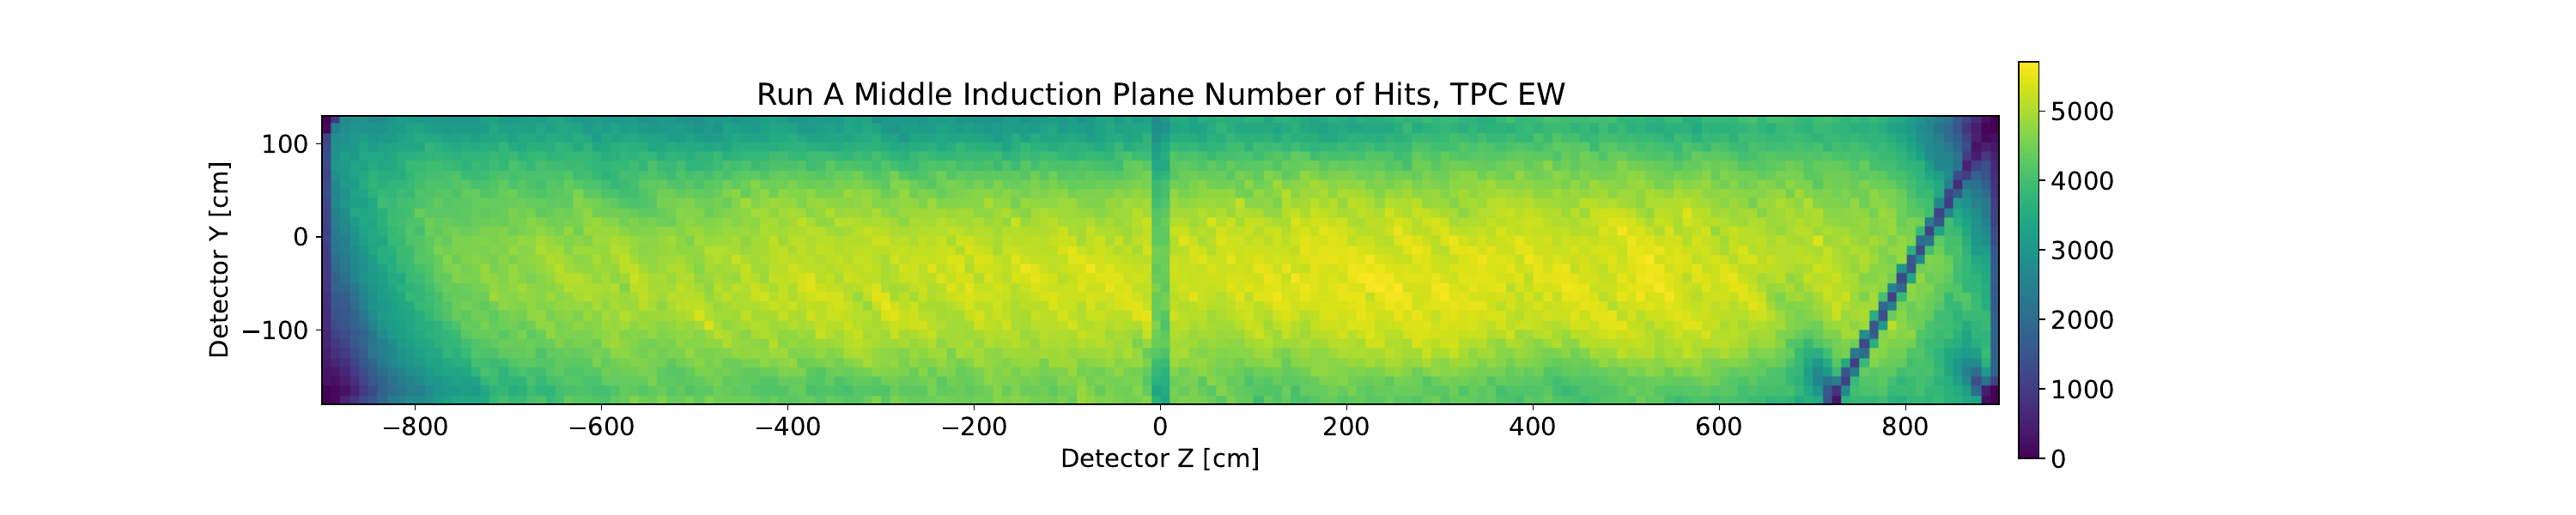}
    \includegraphics[width=\textwidth]{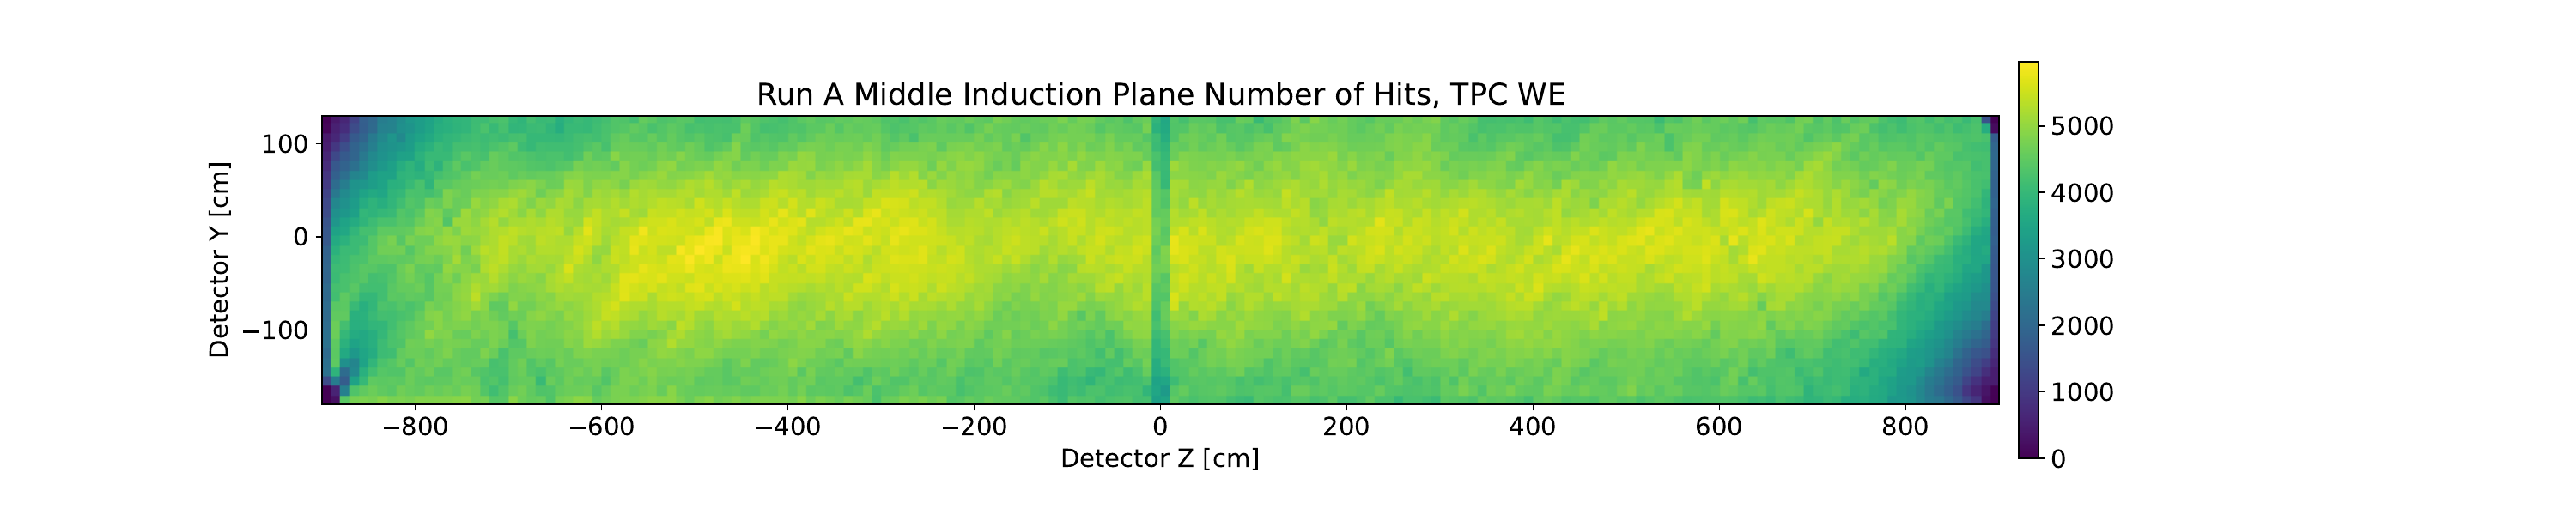}
    \includegraphics[width=\textwidth]{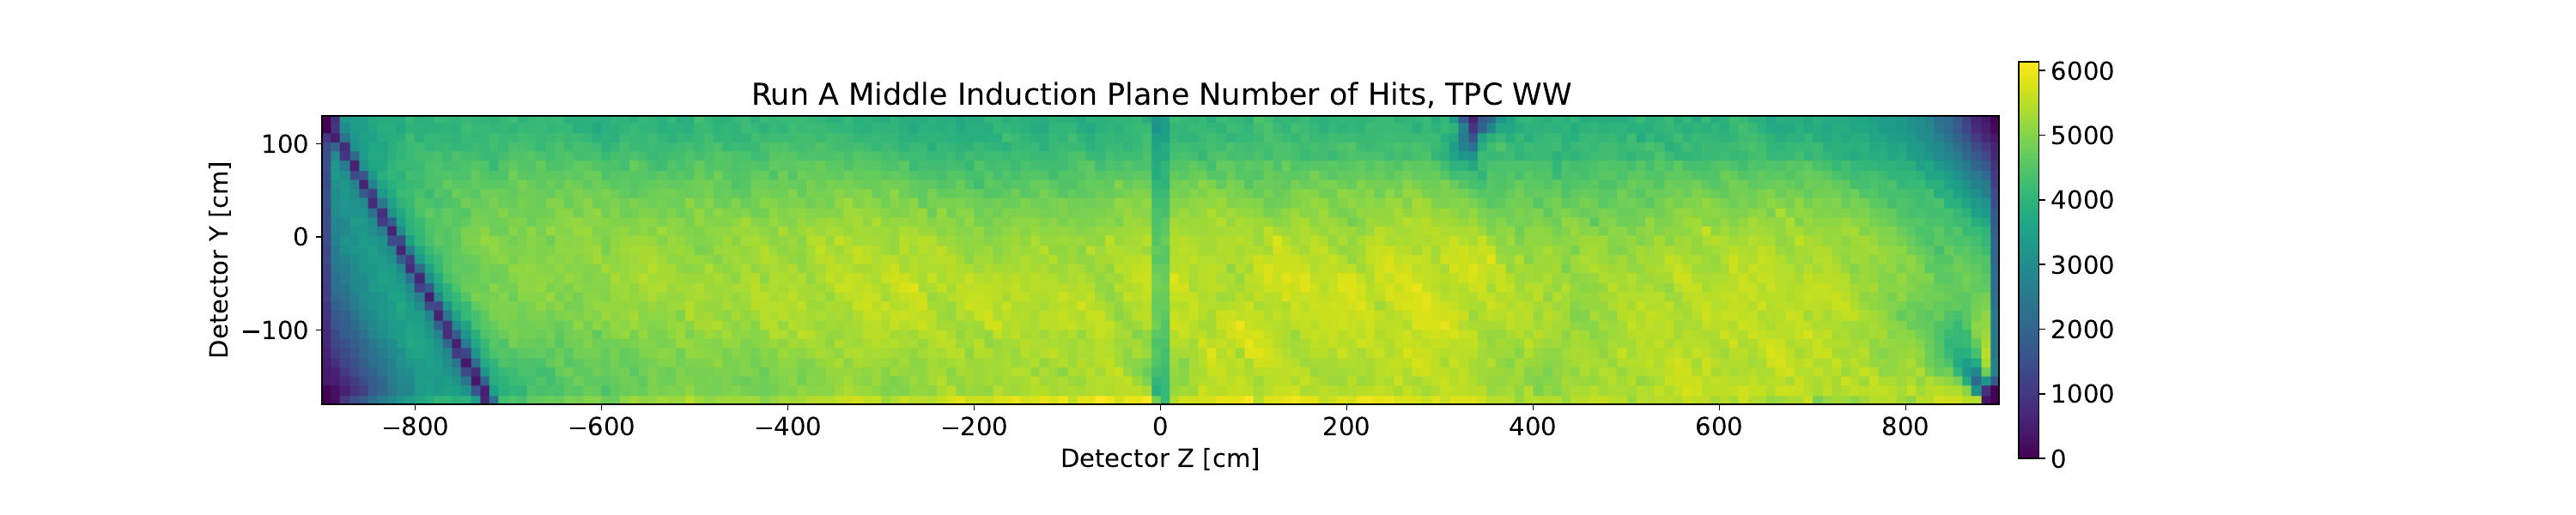}
    \caption{Number of depositions in $10\times$\SI{10}{\centi\meter} bins in each of the ICARUS TPCs on the middle induction plane across the Run A dataset.}
    \label{fig:w=runAInd1N}
\end{figure}

\begin{figure}[]
    \centering
    \includegraphics[width=\textwidth]{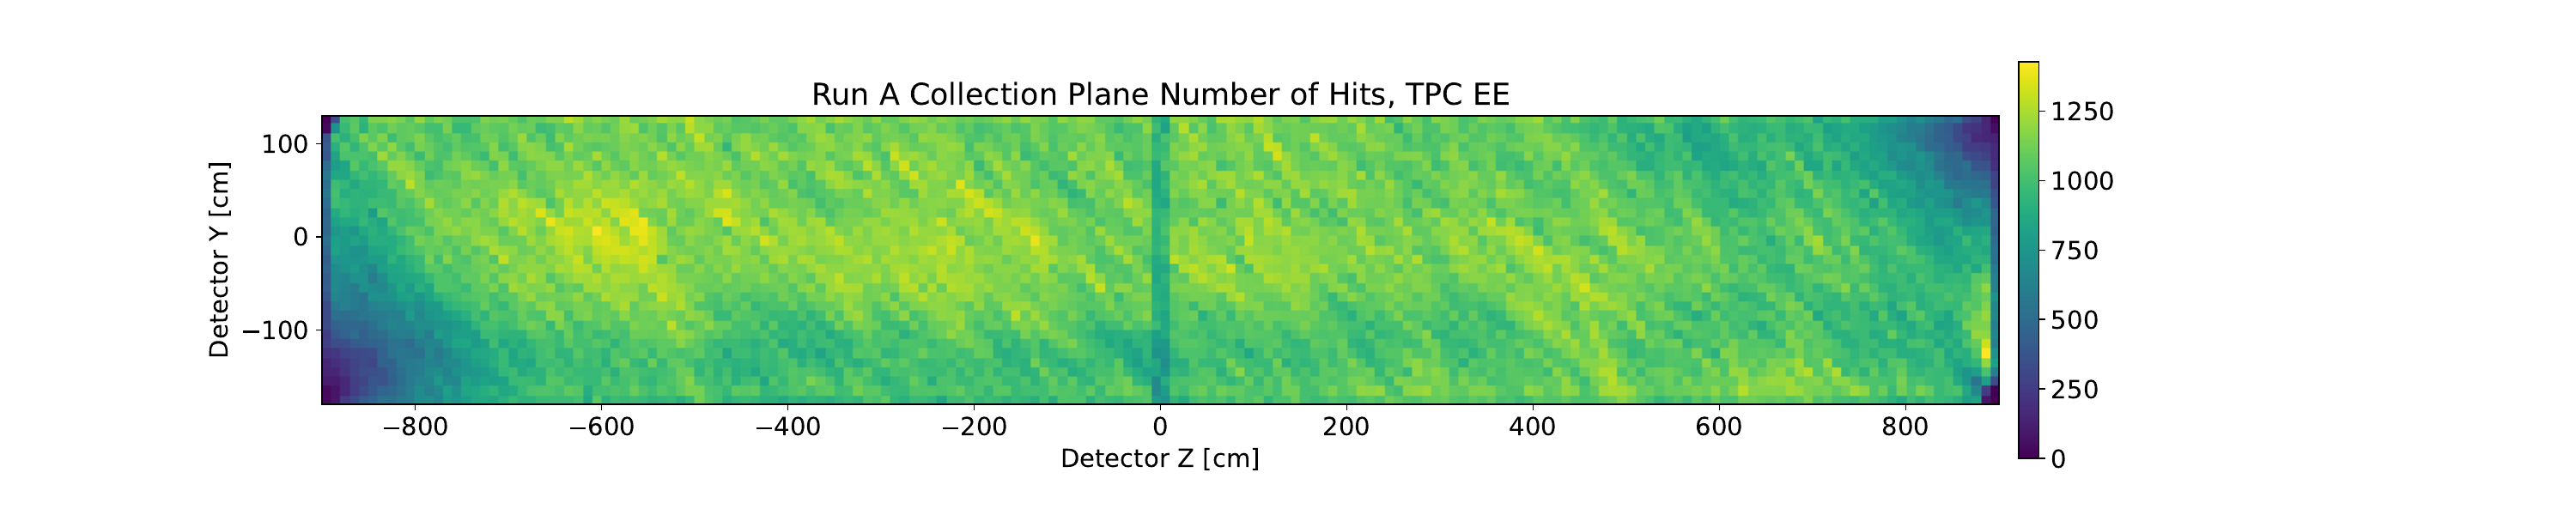}
    \includegraphics[width=\textwidth]{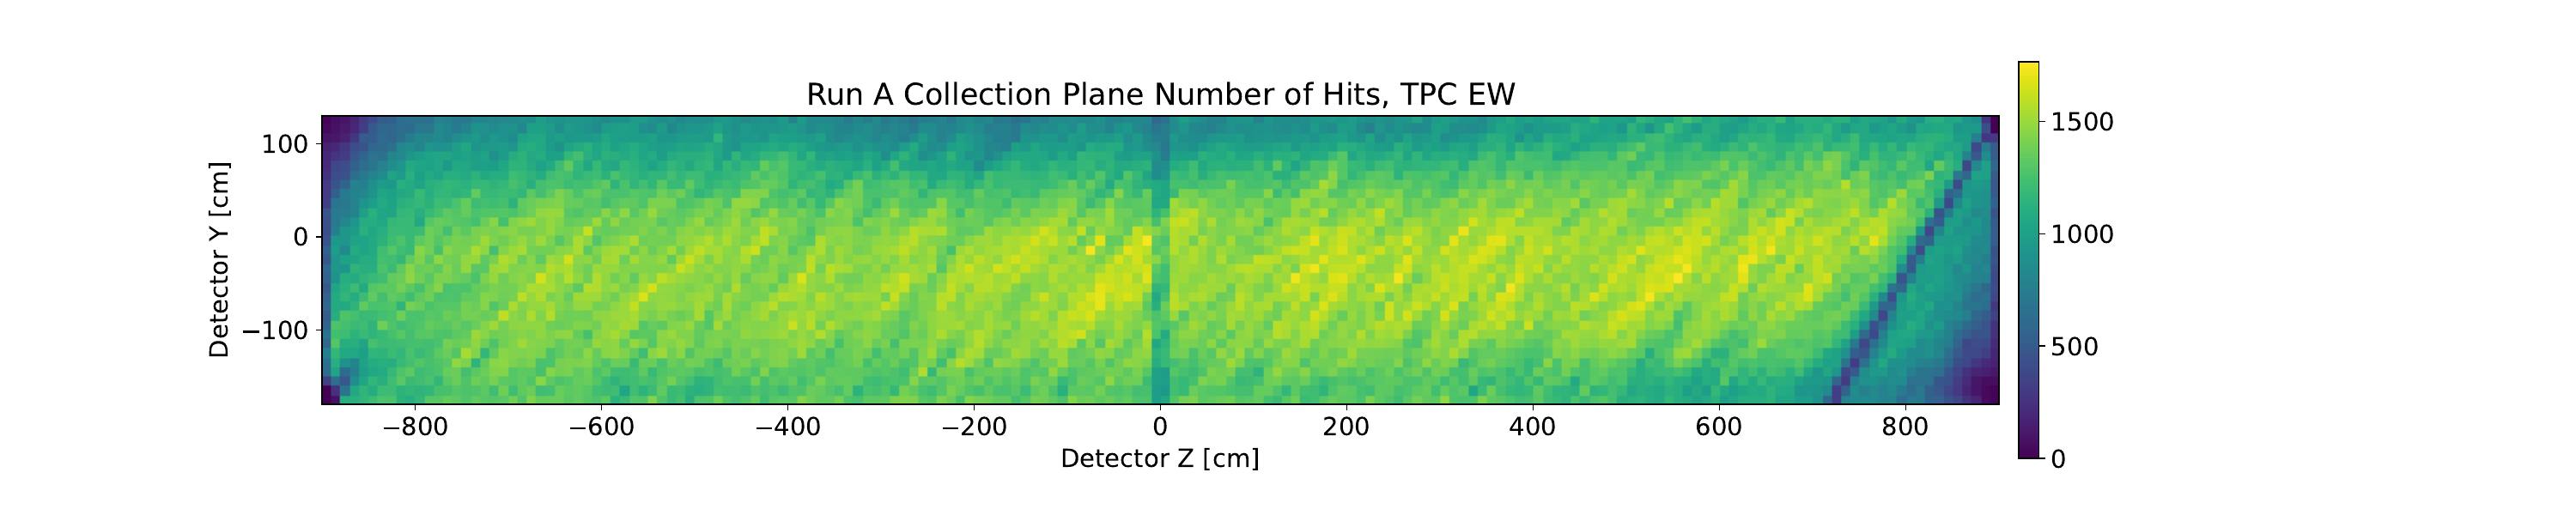}
    \includegraphics[width=\textwidth]{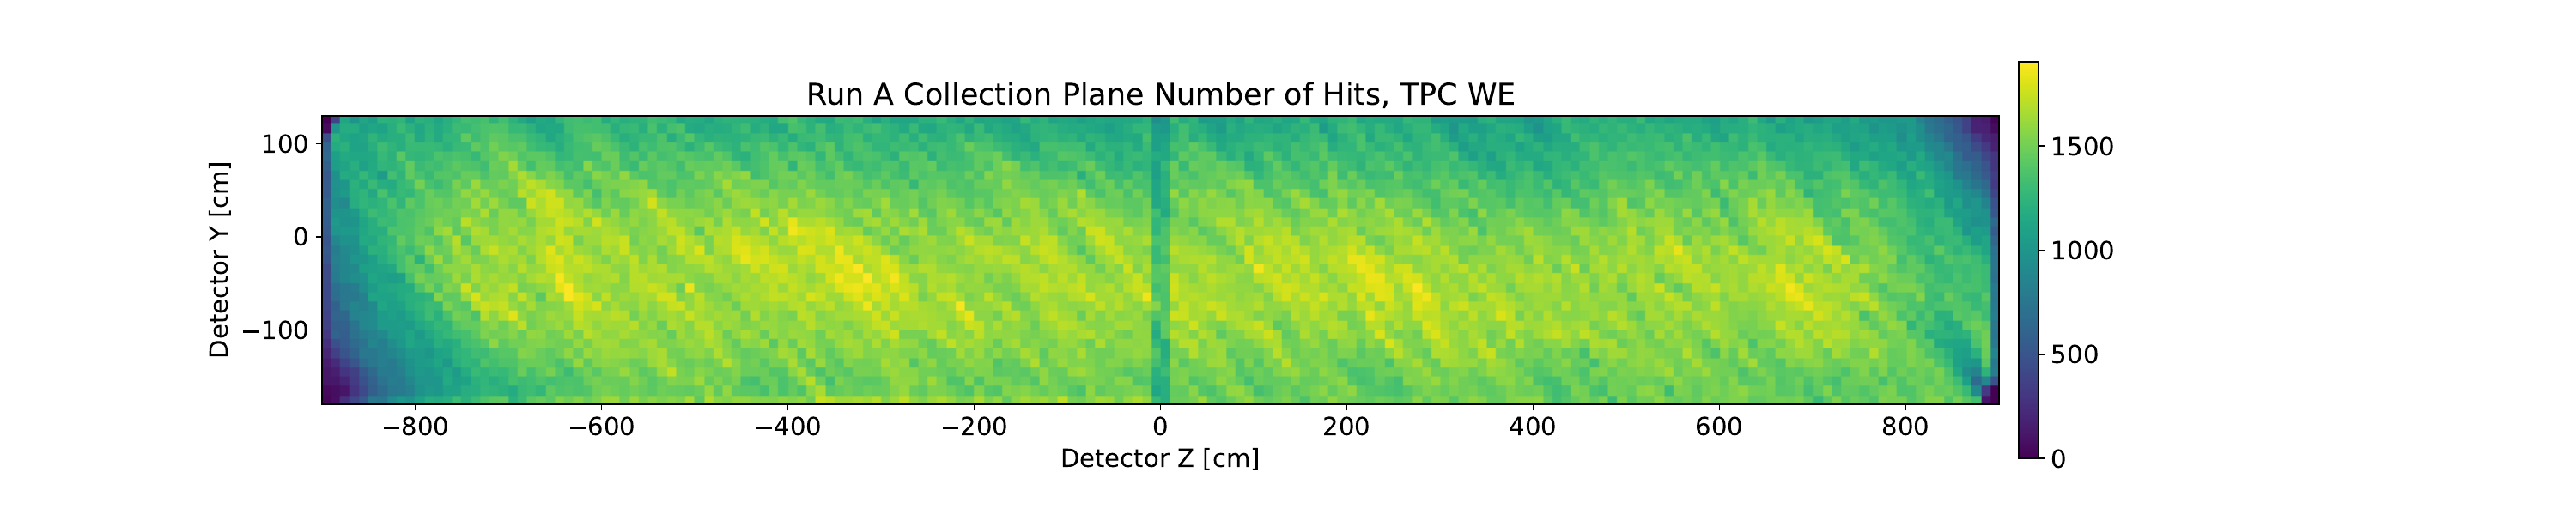}
    \includegraphics[width=\textwidth]{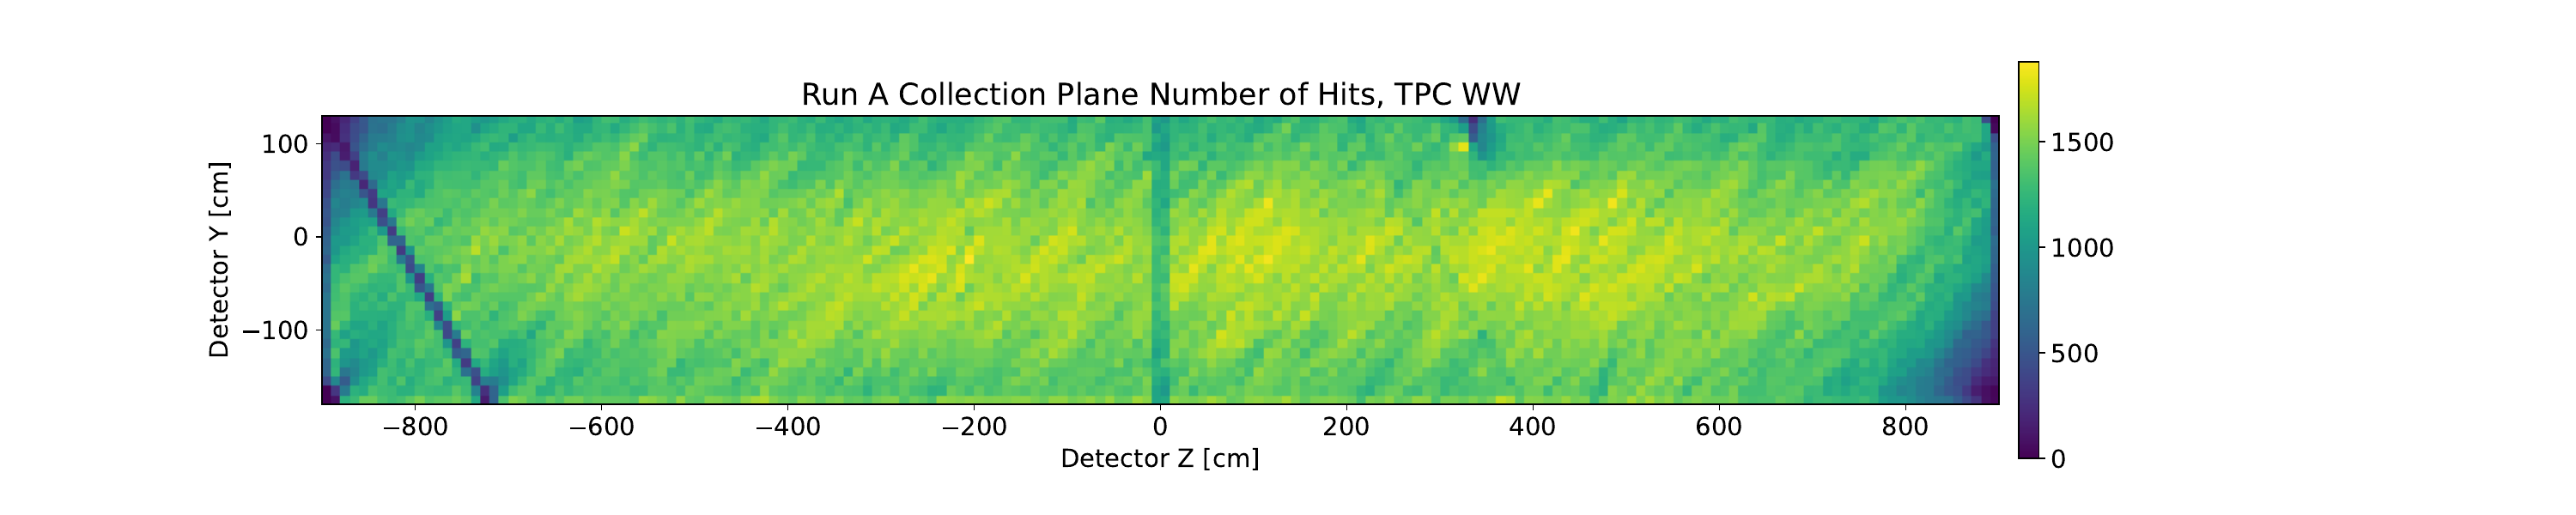}
    \caption{Number of depositions in $10\times$\SI{10}{\centi\meter} bins in each of the ICARUS TPCs on the collection plane across the Run A dataset.}
    \label{fig:w=runAColN}
\end{figure}

\begin{figure}[]
    \centering
    \includegraphics[width=\textwidth]{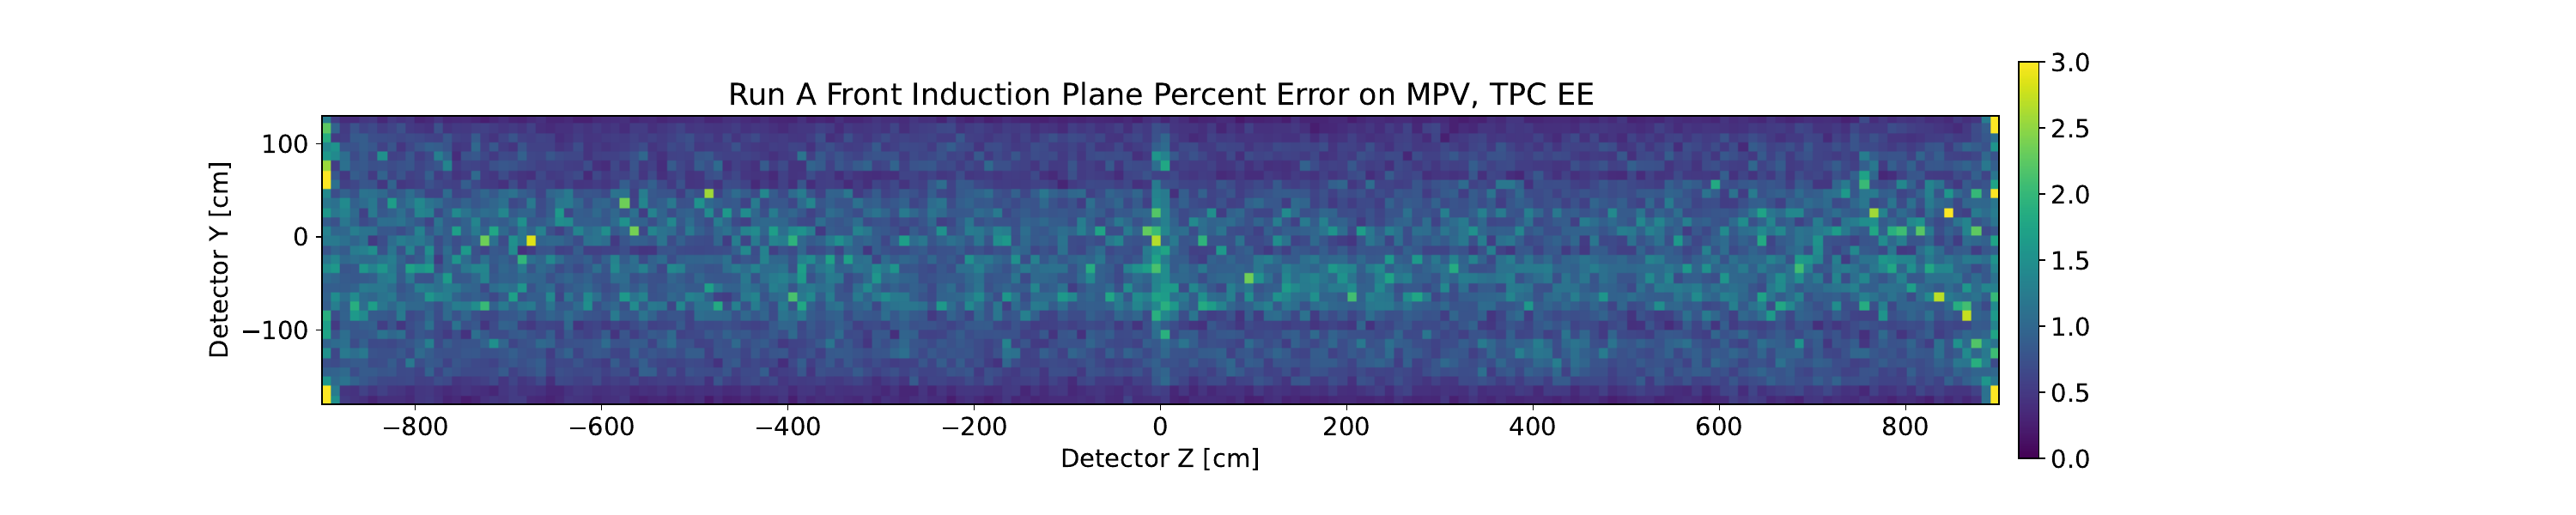}
    \includegraphics[width=\textwidth]{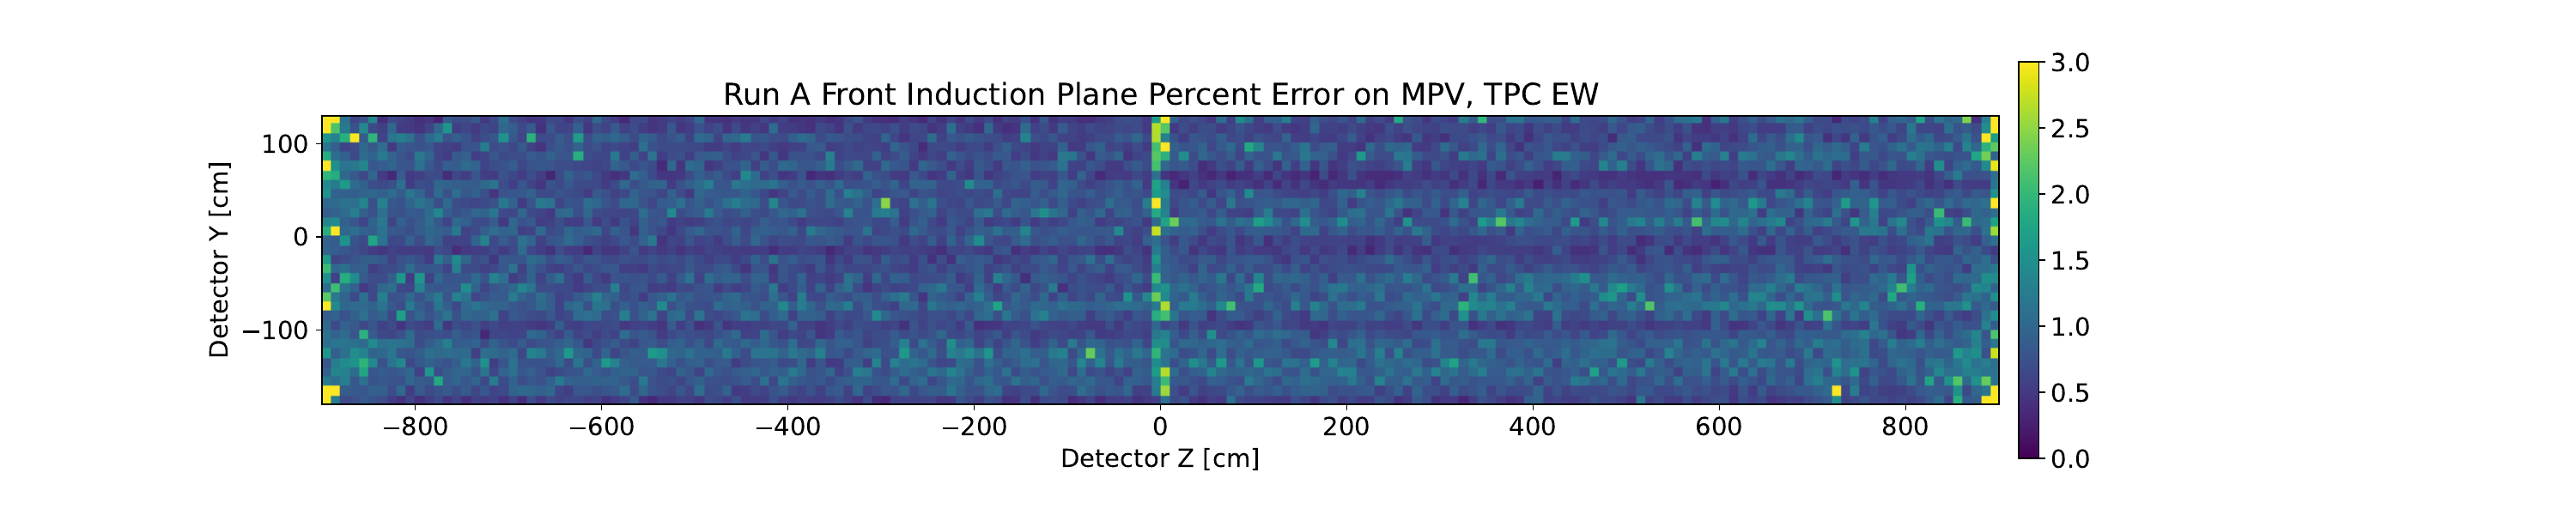}
    \includegraphics[width=\textwidth]{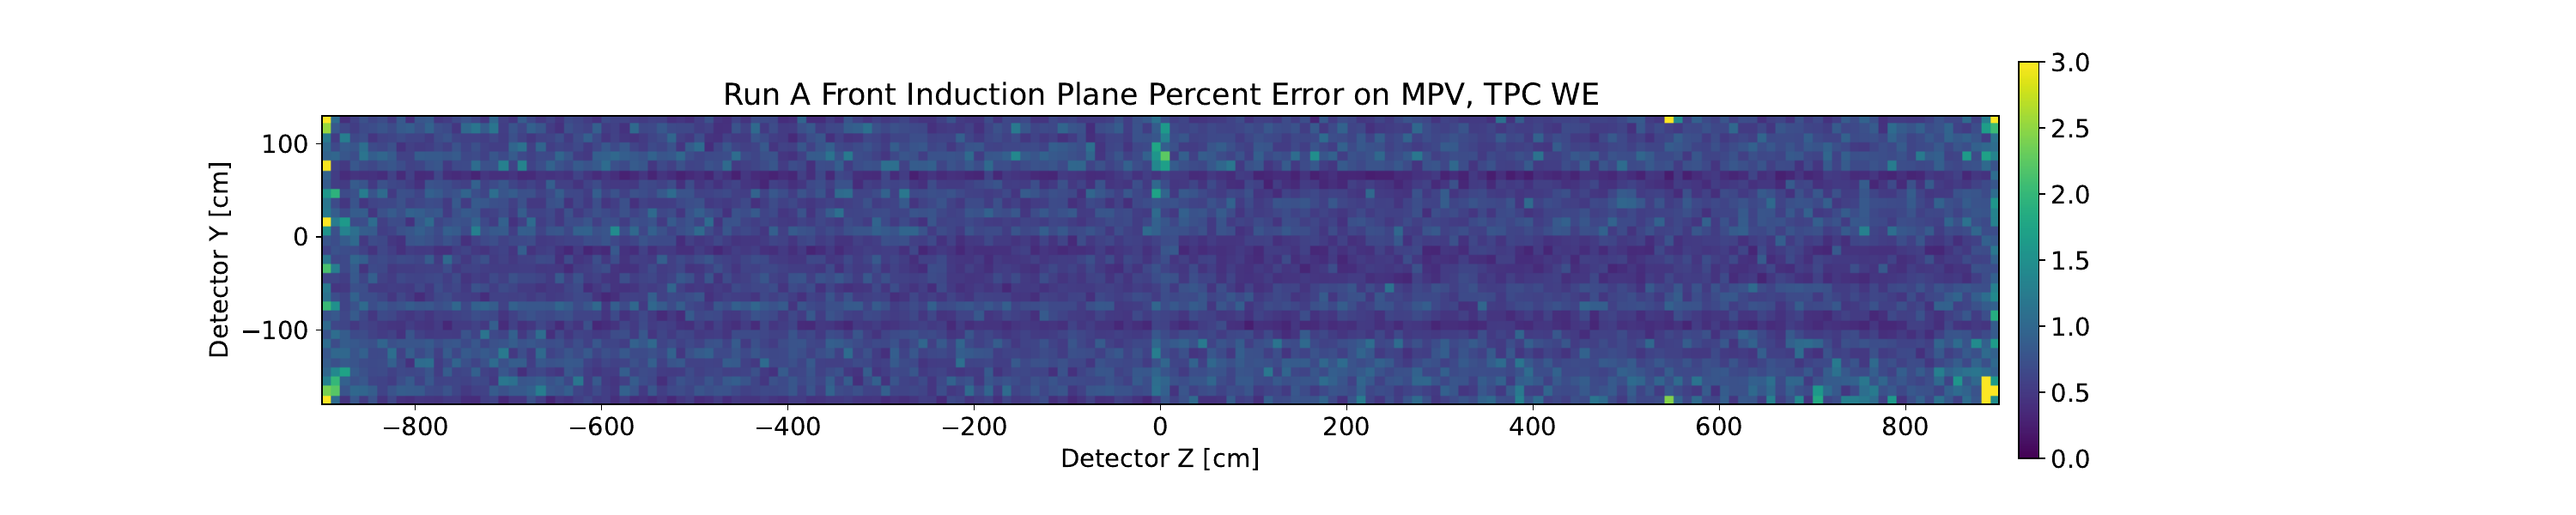}
    \includegraphics[width=\textwidth]{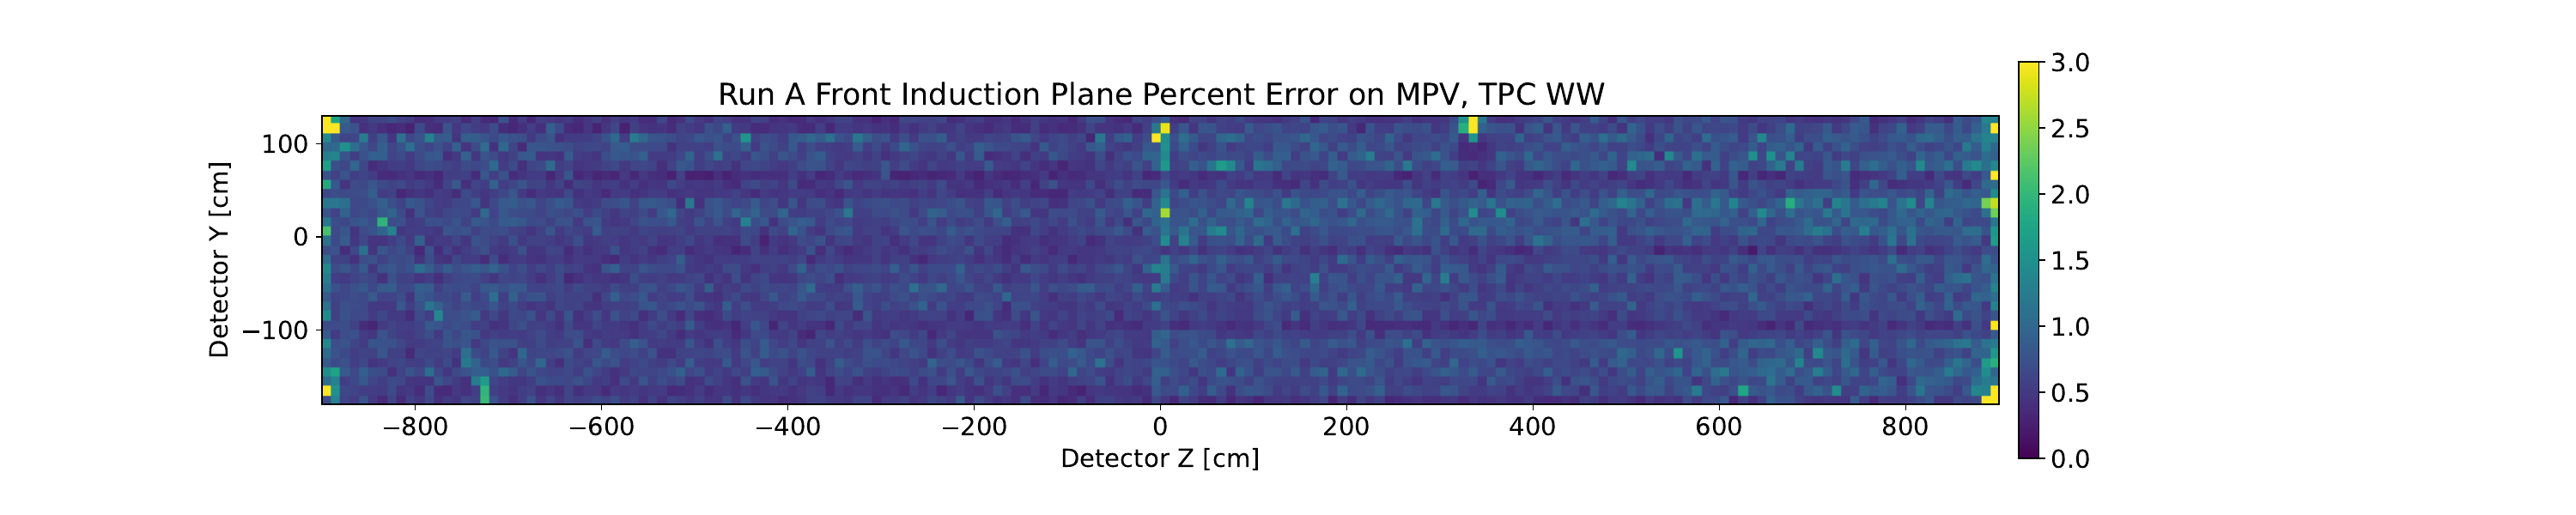}
    \caption{Error on the MPV $dQ/dx$ in $10\times$\SI{10}{\centi\meter} bins in each of the ICARUS TPCs on the front induction plane across the Run A dataset.}
    \label{fig:w=runAInd0Err}
\end{figure}

\begin{figure}[]
    \centering
    \includegraphics[width=\textwidth]{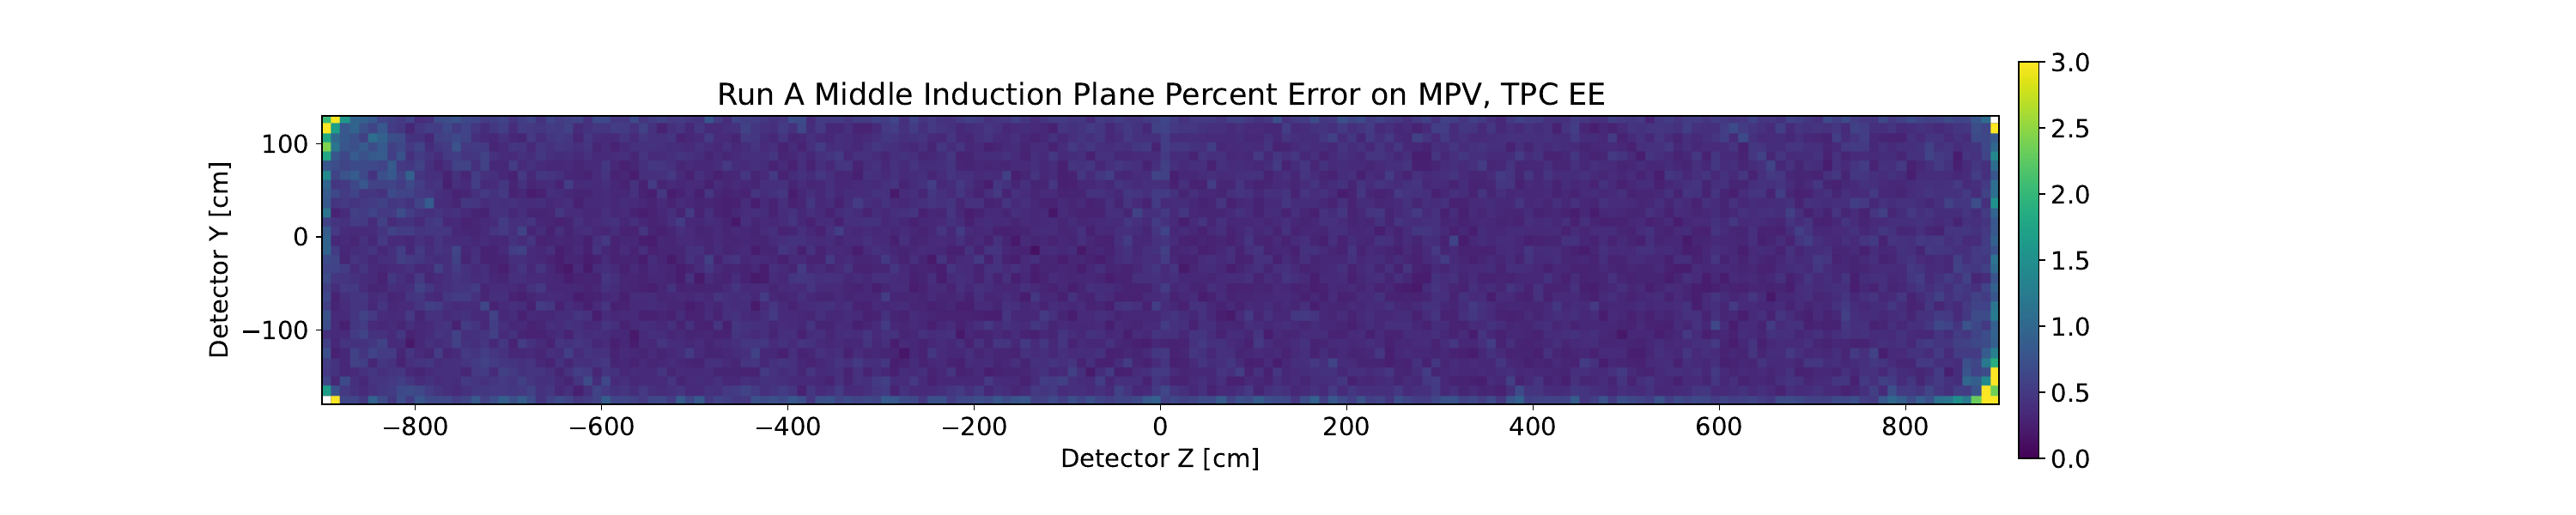}
    \includegraphics[width=\textwidth]{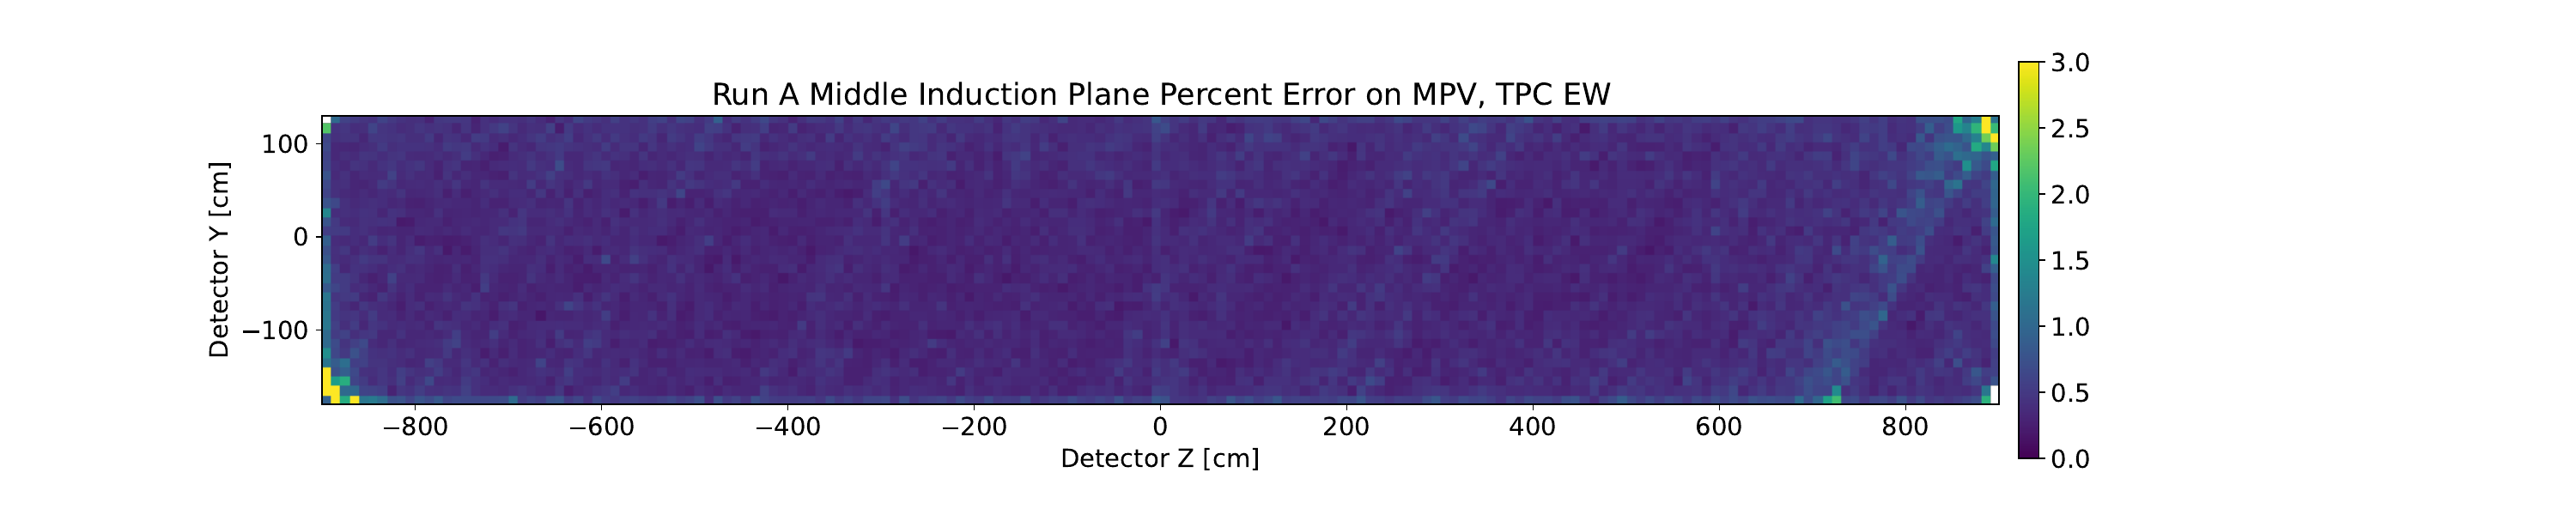}
    \includegraphics[width=\textwidth]{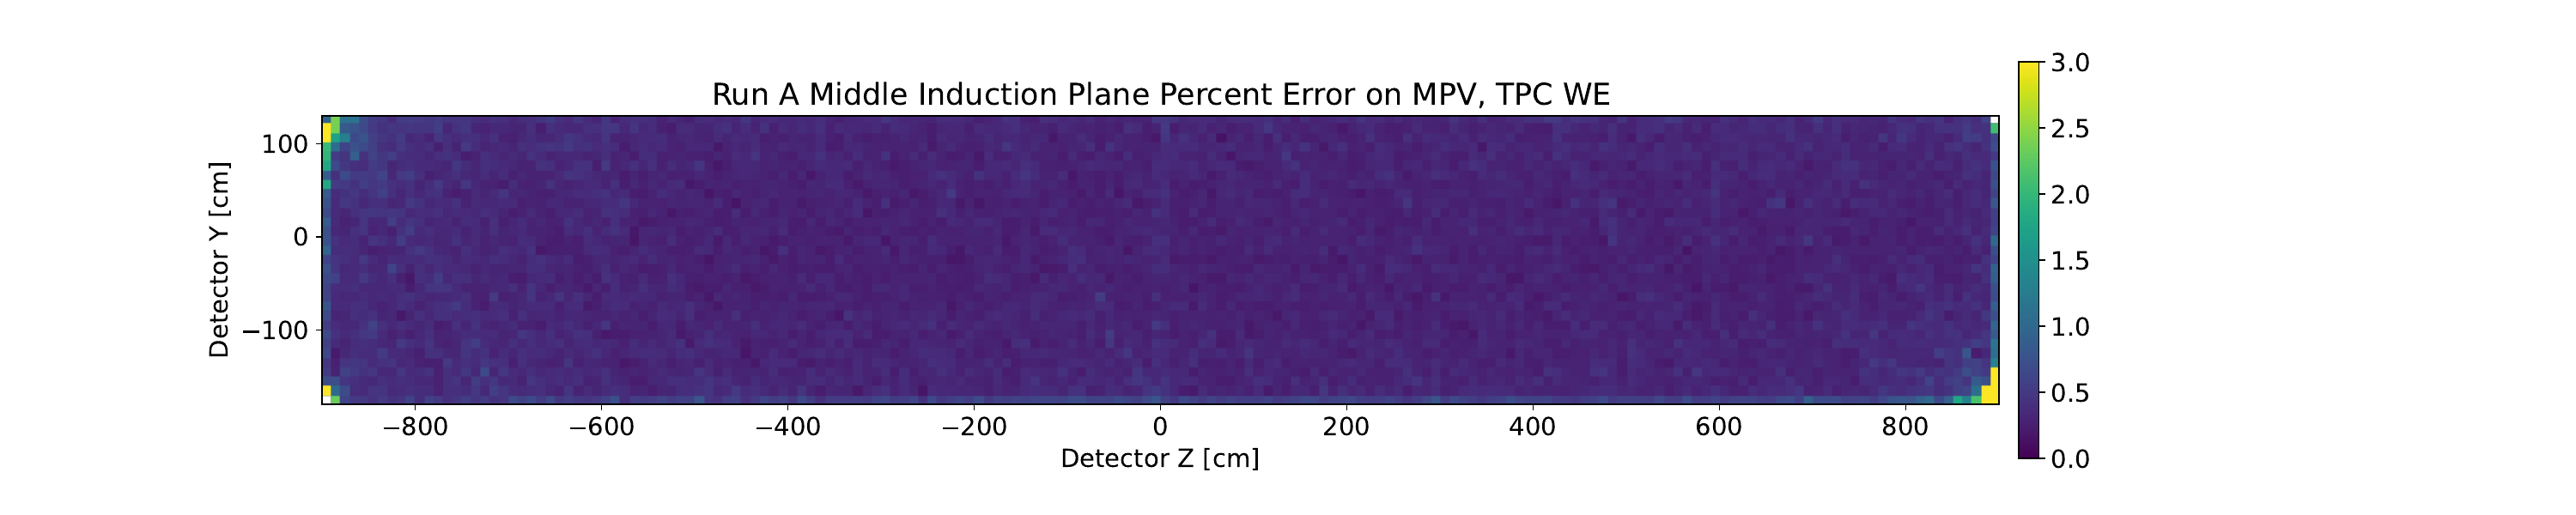}
    \includegraphics[width=\textwidth]{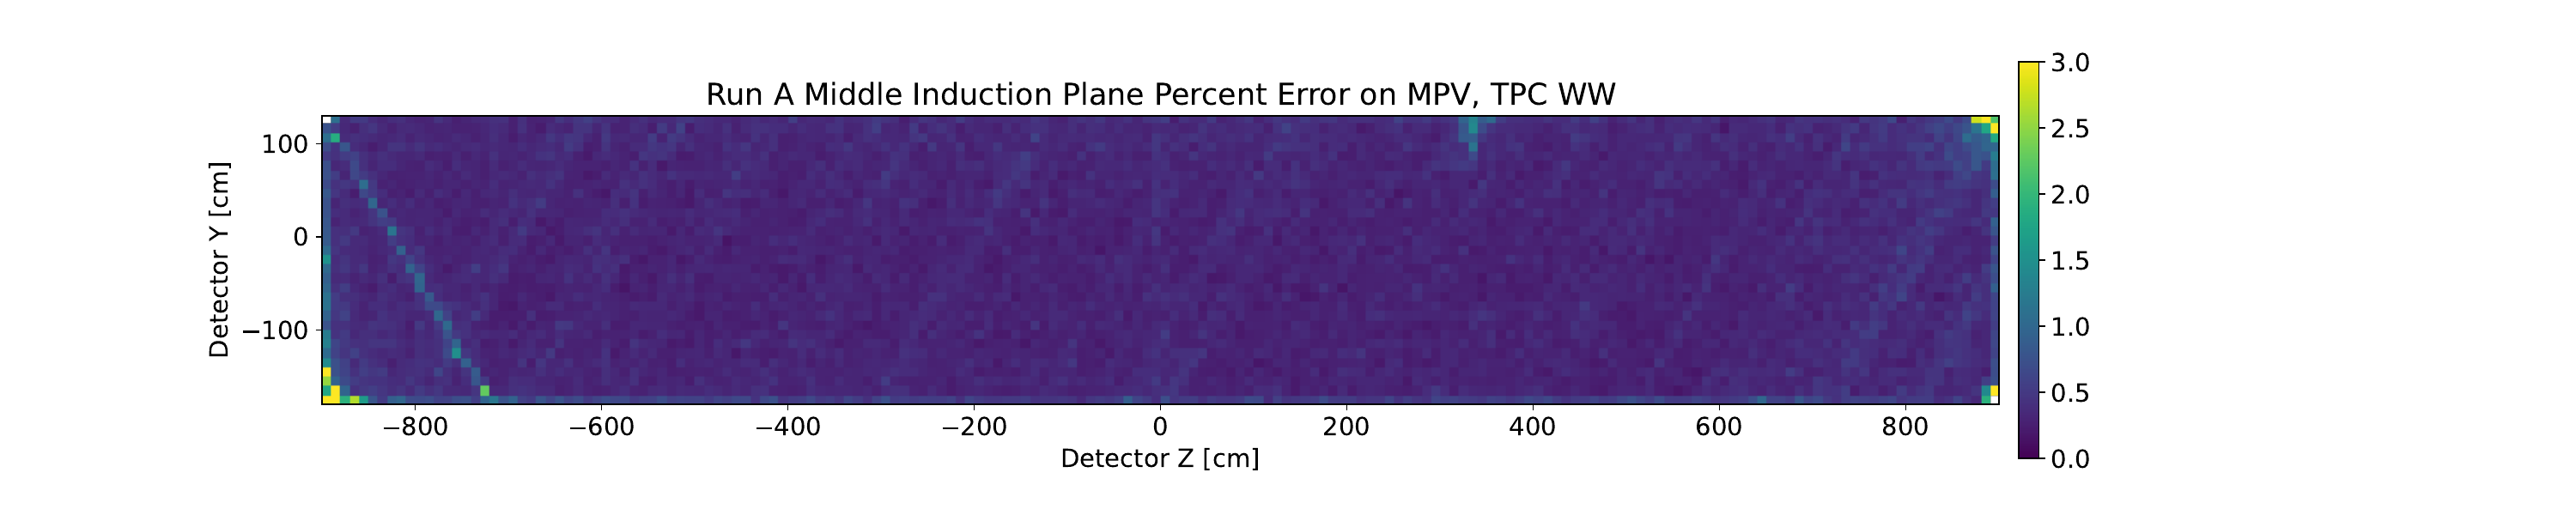}
    \caption{Error on the MPV $dQ/dx$ in $10\times$\SI{10}{\centi\meter} bins in each of the ICARUS TPCs on the middle induction plane across the Run A dataset.}
    \label{fig:w=runAInd1Err}
\end{figure}

\begin{figure}[]
    \centering
    \includegraphics[width=\textwidth]{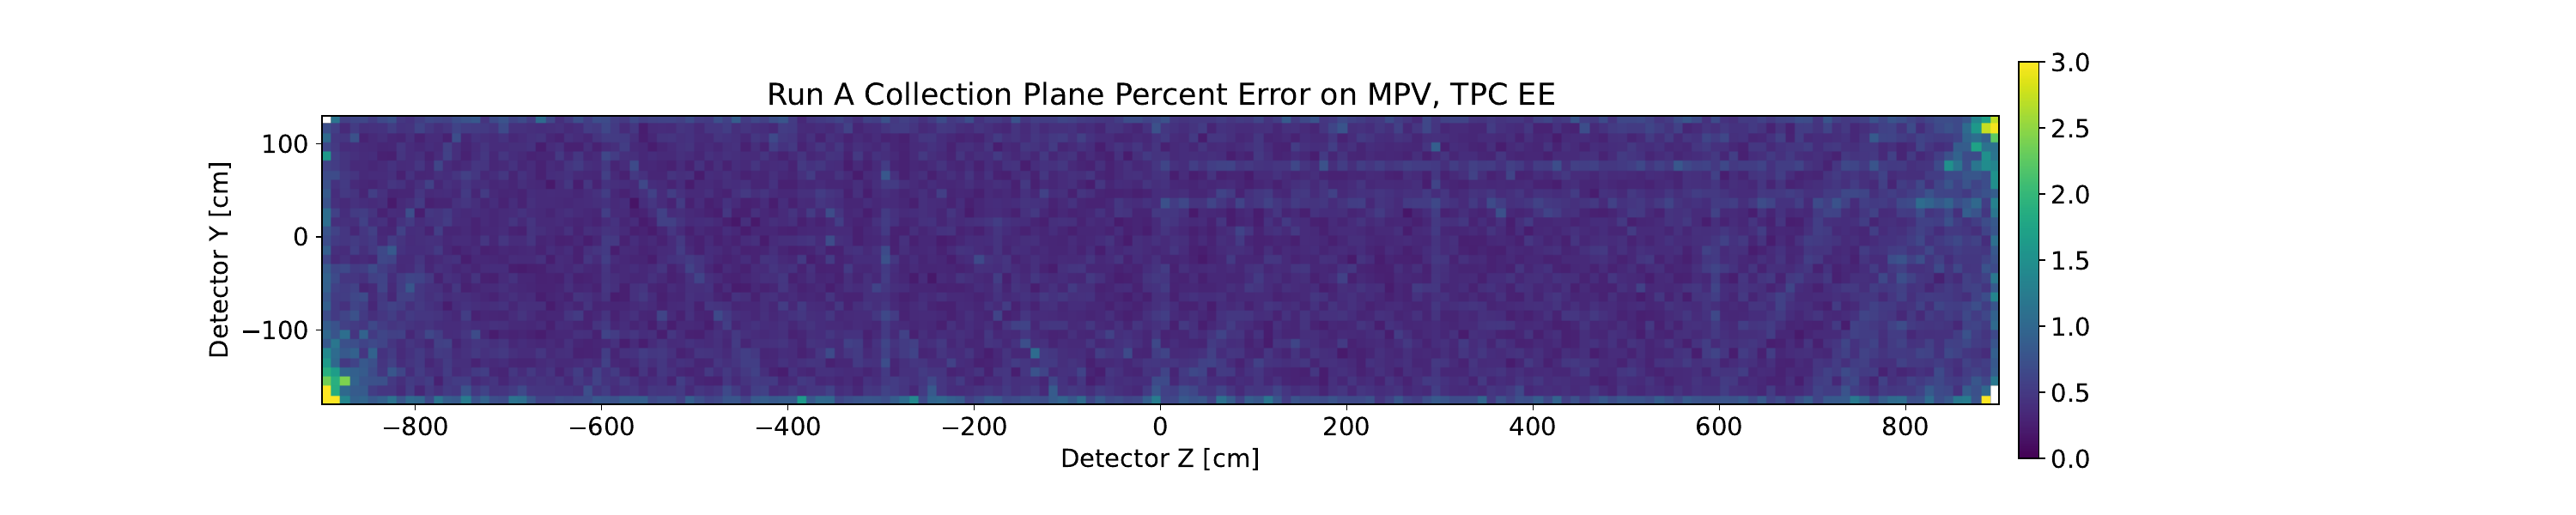}
    \includegraphics[width=\textwidth]{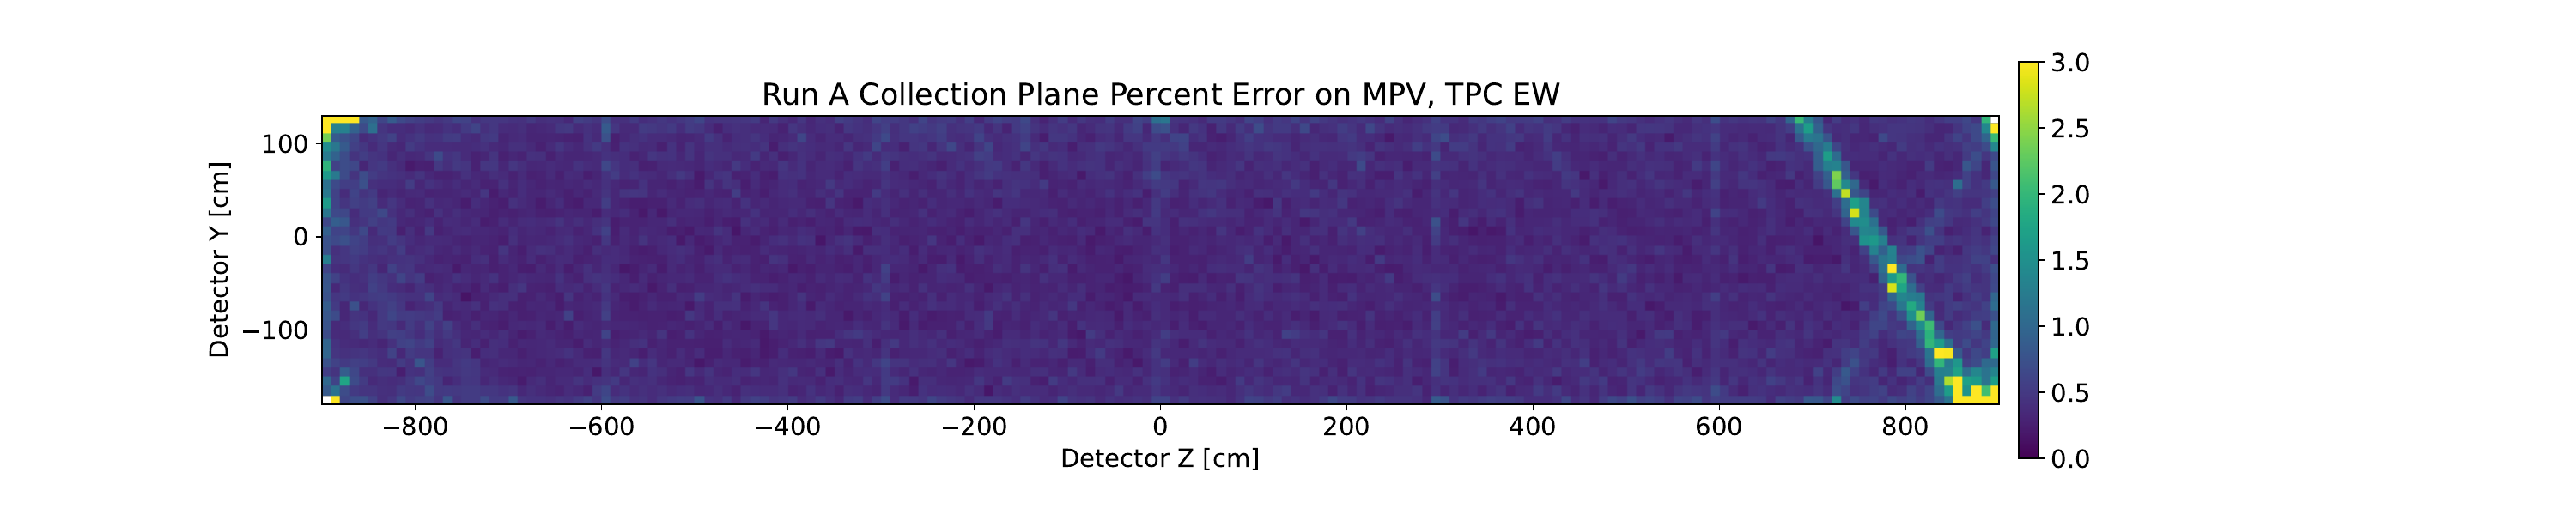}
    \includegraphics[width=\textwidth]{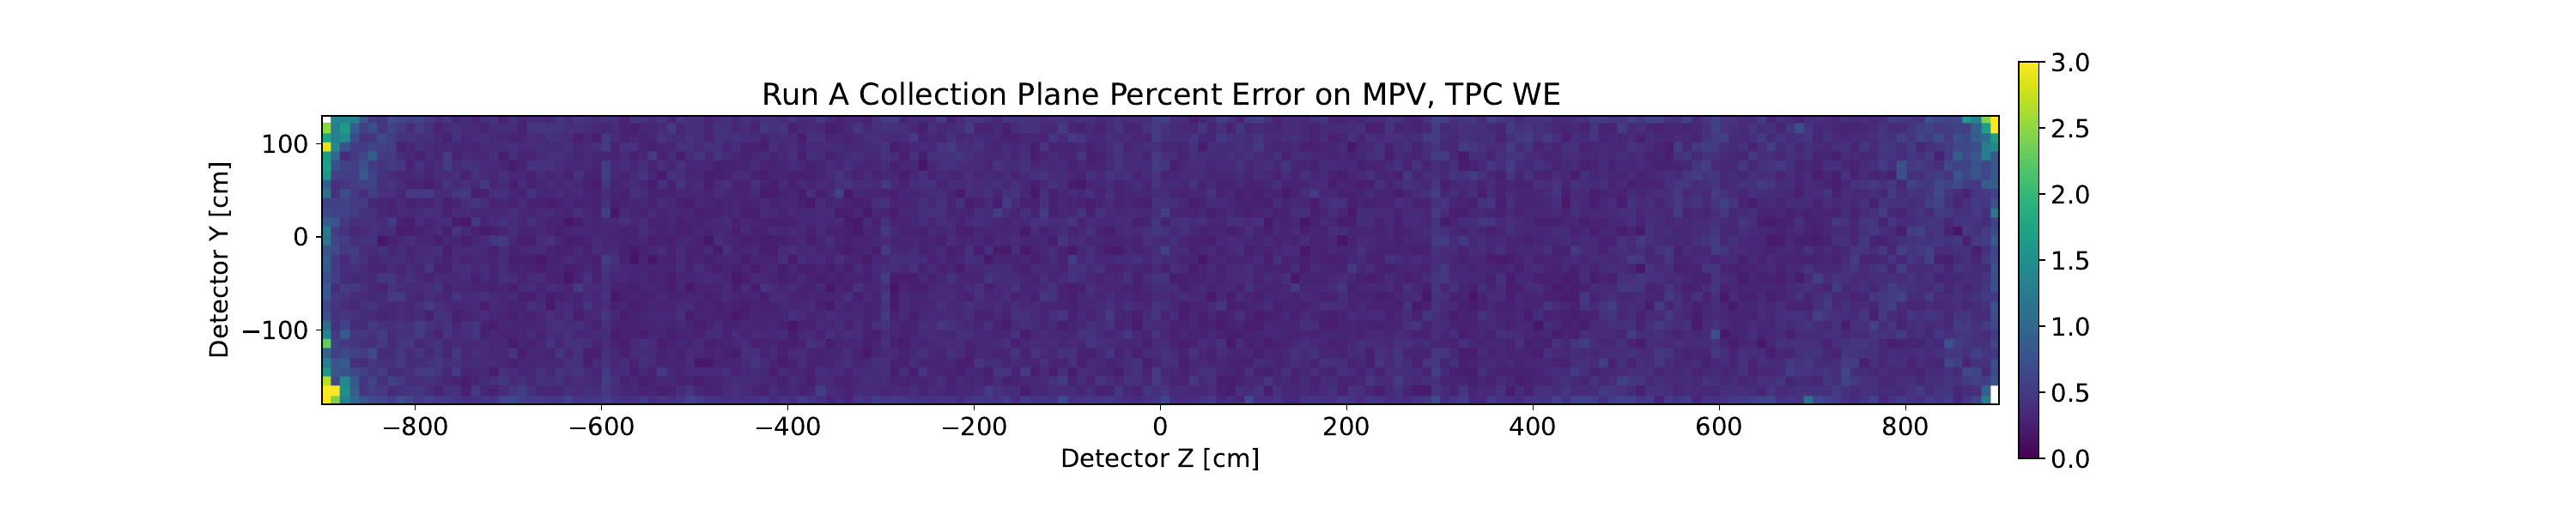}
    \includegraphics[width=\textwidth]{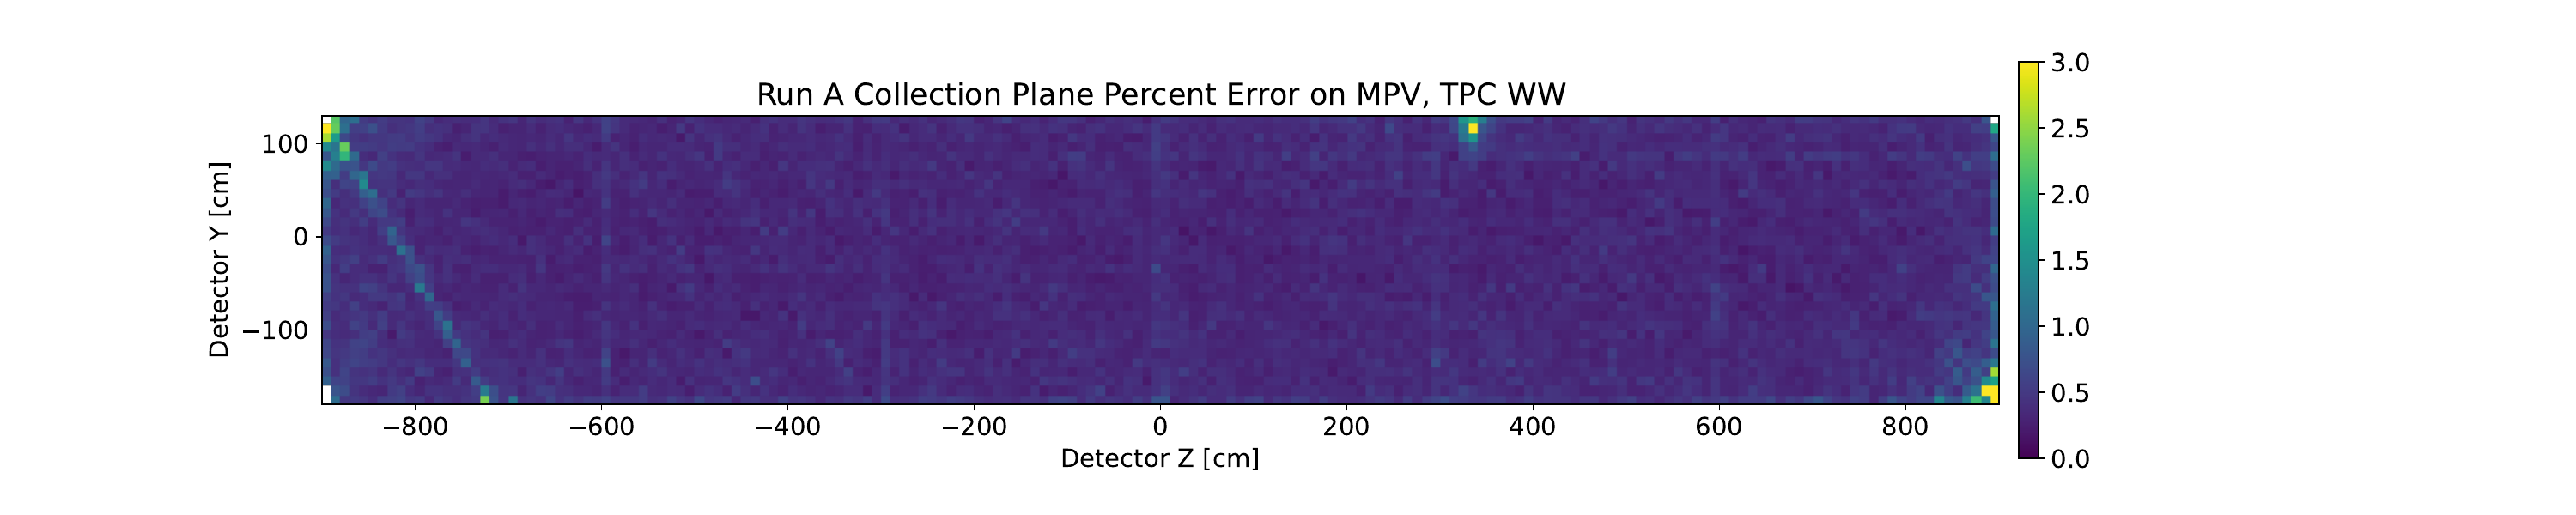}
    \caption{Error on the MPV $dQ/dx$ in $10\times$\SI{10}{\centi\meter} bins in each of the ICARUS TPCs on the collection plane across the Run A dataset.}
    \label{fig:w=runAColErr}
\end{figure}

The number of depositions on each plane is shown in figures \ref{fig:w=runAInd0N}, \ref{fig:w=runAInd1N}, and \ref{fig:w=runAColN}. The percent uncertainty on the MPV on each plane is shown in figures \ref{fig:w=runAInd0Err}, \ref{fig:w=runAInd1Err}, and \ref{fig:w=runAColErr}. Most notably, there are two bands, one in TPC EW and one in TPC WW, where there is a deficit of depositions on each plane. On the collection plane, these two regions also have a much larger percent error on the MPV. Both regions are bands in the direction of the collection plane wires in that TPC. The version of reconstruction used to identify cosmic muon tracks for this study required hits to be identified across all three planes, so the dearth of hits on the other two planes could be an artifact of this reconstruction. It is not known what the issue on the collection plane though could be.
